# Supplementary material for: m-Nearly k-Universal Words -- Investigating Simon Congruence
Source: arXiv:2202.07981 source file (2022-02-16)
Supplement: Supplementary file 1 [file proof-add_arches.tex]

\begin{proof}
		(i) Let $\tilde{w} = \operatorname{arch} \cdot w$ and $\tx \notin \alph(\r(w))$, then all scattered factors of $w$ are in $\tilde{w}$. Because we need scattered factors of length $k+1$, we expand each scattered factor with each letter in $\operatorname{arch}$. Thus, we have $\vert \Sigma \vert \cdot (\vert \Sigma \vert^k - 1) = \vert \Sigma \vert^{k+1} - \vert \Sigma \vert$ scattered factors of length $k+1$ in $\tilde{w}$. Consider all scattered factors with last letter $\tx$, because these are $\vert \Sigma \vert$ missing scattered factors in $\tilde{w}$. Because we do not need all of these scatterd factors in $\tilde{w}$, we do not consider the scattered factor, which is $\m(\tilde{w})\tx$. Now we consider only $\vert \Sigma \vert - 1$ scattered factors with last letter $\tx$, which have to be in $\tilde{w}$. Because we have $k-1$ arches in w, we consider only prefixes of length two of these scattered factors. If these prefixes are scattered factors of $\operatorname{arch}$, then $\tilde{w}$ is nearly $(k+1)$-universal. This arch exists, because we can find a permutation of $\operatorname{inner}_1(\operatorname{arch})$ and can use the Paper-Streamer-Method with this permutation by \cite{BAAnni} to get all prefixes as a scattered factor of $\operatorname{arch}$.
		
		(ii) Now let $\tilde{w} = \operatorname{ar}_1(w)$ ... $\operatorname{ar}_i(w) \cdot \operatorname{arch} \cdot$ ... $\operatorname{ar}_{k-1}(w) \operatorname{r}$(w). Like before, we expand all scattered factors, but now at the position $i$. So the scattered factors have the expanded letter at position $i$ and after that they stay the same as before. We also consider the scattered factor with last letter $\tx \notin \alph(\r(w))$. Like before the missing scattered factor $\m(w) [ 1...i ] \m ( \operatorname{arch} ) \m(w)$$ [ i+1...k-1 ] \tx$ has to be the missing scattered factor of $\tilde{w}$. Because $w$ has again $(k-1)$ arches and the scattered factors are expanded after position $i$, we have a look at the factors of these scattered factos after position $i$ of length two. If these factors are scattered factors of $\operatorname{arch}$, then $\tilde{w}$ is nearly $(k+1)$-universal. We find this arch with all factors as scattered factors, because we can find a permutation of $\operatorname{inner}_1(\operatorname{arch})$ and use the Paper-Streamer-Method with this permutation by \cite{BAAnni} to get all prefixes as a scattered factor of $\operatorname{arch}$.
		
		(iii) Let $\tilde{w} = \operatorname{ar}_1(w)$ ... $\operatorname{ar}_{k-1}(w) \cdot \operatorname{arch} \cdot \operatorname{r}(w)$. With the same argument like in (ii), we expand the scattered factors after the position $k-1$. Then we consider the scattered factor with last letter $\tx \notin \alph(\r(w))$ and consider the factors of length two at position $k-1$ and $k$ of the expanded scattered factors. If these factors are in arch, then $\tilde{w}$ is nearly $(k+1)$-universal and we get these factors in arch, because we can find a permutation of $\operatorname{inner}_1(\operatorname{arch})$ and can use the Paper-Streamer-Method with this permutation by \cite{BAAnni} to get all prefixes as a scattered factor of $\operatorname{arch}$.
	
\end{proof}
