# Supplementary material for: m-Nearly k-Universal Words -- Investigating Simon Congruence
Source: arXiv:2202.07981 source file (2022-02-16)
Supplement: Supplementary file 2 [file proof-cutoff_reversedarch.tex]

\begin{proof}

\end{proof}
