# Supplementary material for: m-Nearly k-Universal Words -- Investigating Simon Congruence
Source: arXiv:2202.07981 source file (2022-02-16)
Supplement: Supplementary file 3 [file proof-cutofffirstarch.tex]

\begin{proof}
	Consider the scattered factors with first letter $\m(w[1])$, because the second letter of these scattered factors does not appear twice in the first arch. So these scattered factors are in $\operatorname{ar}_2(w)$ ... $\operatorname{ar}_k-1(w)\r(w)$. The number of these scatterd facotors is $\frac{1}{\vert \Sigma \vert}\vert \Sigma \vert^k - 1$, because one of these scattered factor has the form $\m(w)\tx$ with $\tx \notin \alph(\r(w))$. If we cut off the first letter of these scattered factors, we have $\frac{1}{\vert \Sigma \vert}\vert \Sigma \vert^k - 1 = \vert \Sigma \vert^{k-1}  - 1$ different scattered factors of length $k-1$ in $\operatorname{ar}_2(w)$ ... $\operatorname{ar}_k-1(w)\r(w)$, because the first letter of all these scatterd factors were the same. Therefore $\operatorname{ar}_2(w)$ ... $\operatorname{ar}_k-1(w)\r(w)$ is nearly $(k-1)$-universal.
\end{proof}
