# Supplementary material for: m-Nearly k-Universal Words -- Investigating Simon Congruence
Source: arXiv:2202.07981 source file (2022-02-16)
Supplement: Supplementary file 4 [file proof-wwR_nearly.tex]

\begin{proof}
We consider $\r(w)\r(w)^R$, which is the middle part in $ww^R$. Because $\alph(\r(w))= \alph(\r(w)^R) $ and $\vert \Sigma \vert - 1 = \vert \alph(\r(w)) \vert = \vert \alph(\r(w)^R) \vert$, we define $x = \r(w)\r(w)^R$. Then let $u = \operatorname{ar}_1(w)...\operatorname{ar}_{k-1}(w)$ and $v = \operatorname{ar}_1(w^R)...\operatorname{ar}_{k-1}(w^R)$, so the $uxv^R$-Therorem by \cite{BAAnni} holds and $ww^R$ is nearly $(2k-1)$-universal.
\end{proof}
